# Supplementary material for: VAD360: Viewport Aware Dynamic 360-Degree Video Frame Tiling
Source: arXiv:2105.11563 source file (2021-05-24)
Supplement: Supplementary file 1 [file 10_Appendix.tex]

\clearpage
\section*{Appendix}
\appendix

\section{MNC algorithm}\label{app:mnc}
